# Supplementary material for: Quantum dynamics of coupled excitons and phonons in chain-like systems: tensor train approaches and higher-order propagators
Source: arXiv:2302.03568 source file (2025-01-16)
Supplement: Supplementary file 1 [file TDSE_SI_1.pdf]

# Supporting Information for:
# Quantum dynamics of coupled excitons and phonons in chain-like systems: tensor train approaches and higher-order propagators

Patrick Gelß, Sebastian Matera, Rupert Klein, and Burkhard Schmidt

(Dated: January 16, 2025)

In the main body of the publication, CPU times and approximation qualities for three classes of systems (excitons, phonons, coupled systems) are displayed in Figs. 3–6. However, not all our results could be shown there for reasons of clarity. Hence, in the present *Supporting Information* we include additional figures showing the results for all of the propagation schemes investigated in our study.

## SPLITTING SCHEMES

Figures 1–4 include all variants of splitting schemes investigated in the present work. In addition to the 2nd order Strang-Marchuk (SM) and 8th order Kahan-Li (KL) schemes given already in Figs. 3–6 of the main publication, we show here also results for the 1st order Lie-Trotter (LT) as well as the 4th order Yoshida-Neri (YN) propagators.

## GLOBAL KRYLOV SCHEMES

Figures 5–7 include all variants of global Krylov schemes investigated in the present work. In addition to the 4th order (K4) and 8th order (K8) schemes given already in Figs. 3–6 of the main publication, we show here also results for the 2nd order (K2) as well as the 6th order (K6) propagators.

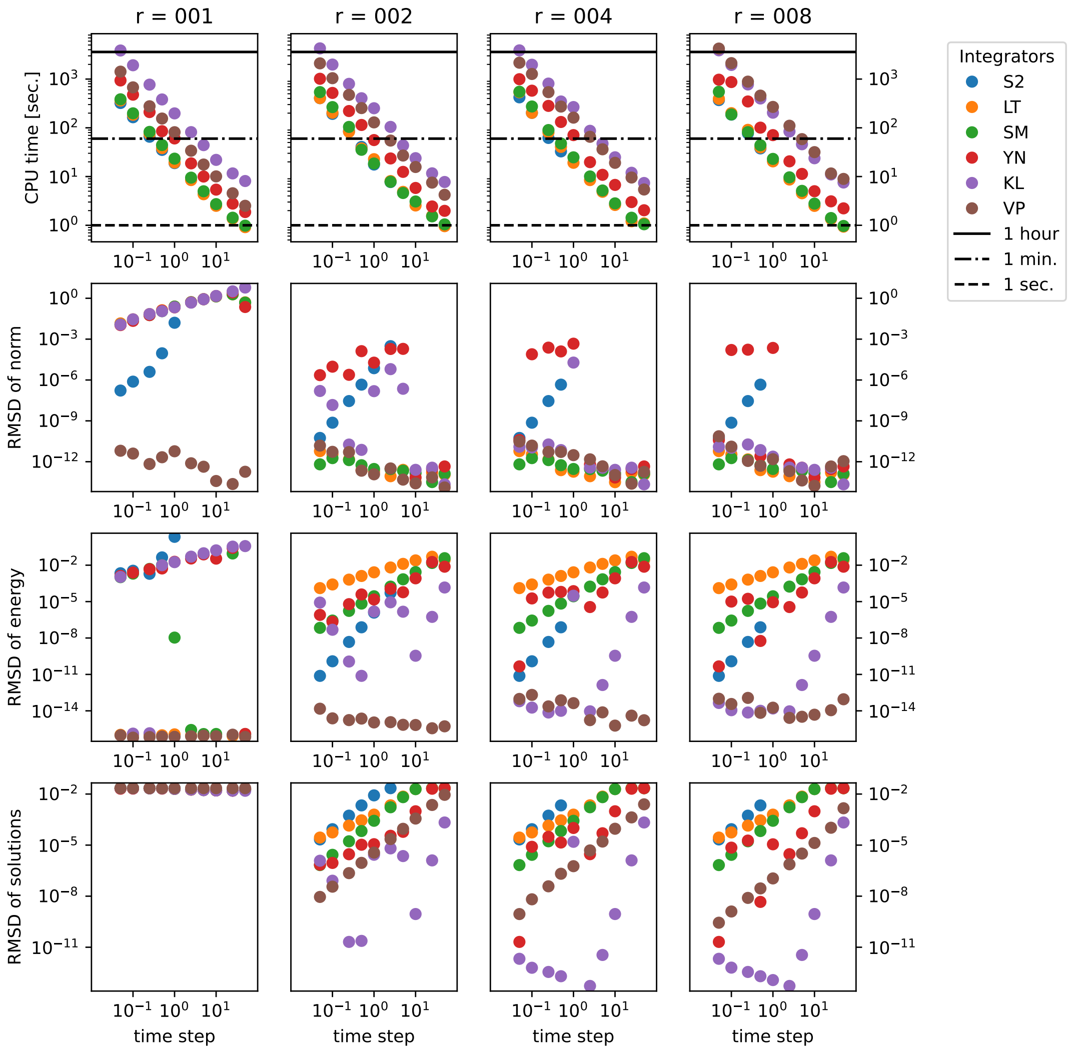


Figure 1. Quantum dynamics of purely excitonic chains with $d = 2$ and $N = 12$ sites. From left to right: Maximum number of ranks of state vectors increasing. From top to bottom: CPU-time versus size of temporal sub-steps, deviation of norm from unity, relative deviation of energy from initial value, deviation of state vectors from semi-analytical reference data. For second order symmetric Euler (S2), Lie-Trotter (LT), Strang-Marchuk (SM), Yoshida-Neri (YN), Kahan-Li (KL), and variational principle (VP) integration methods

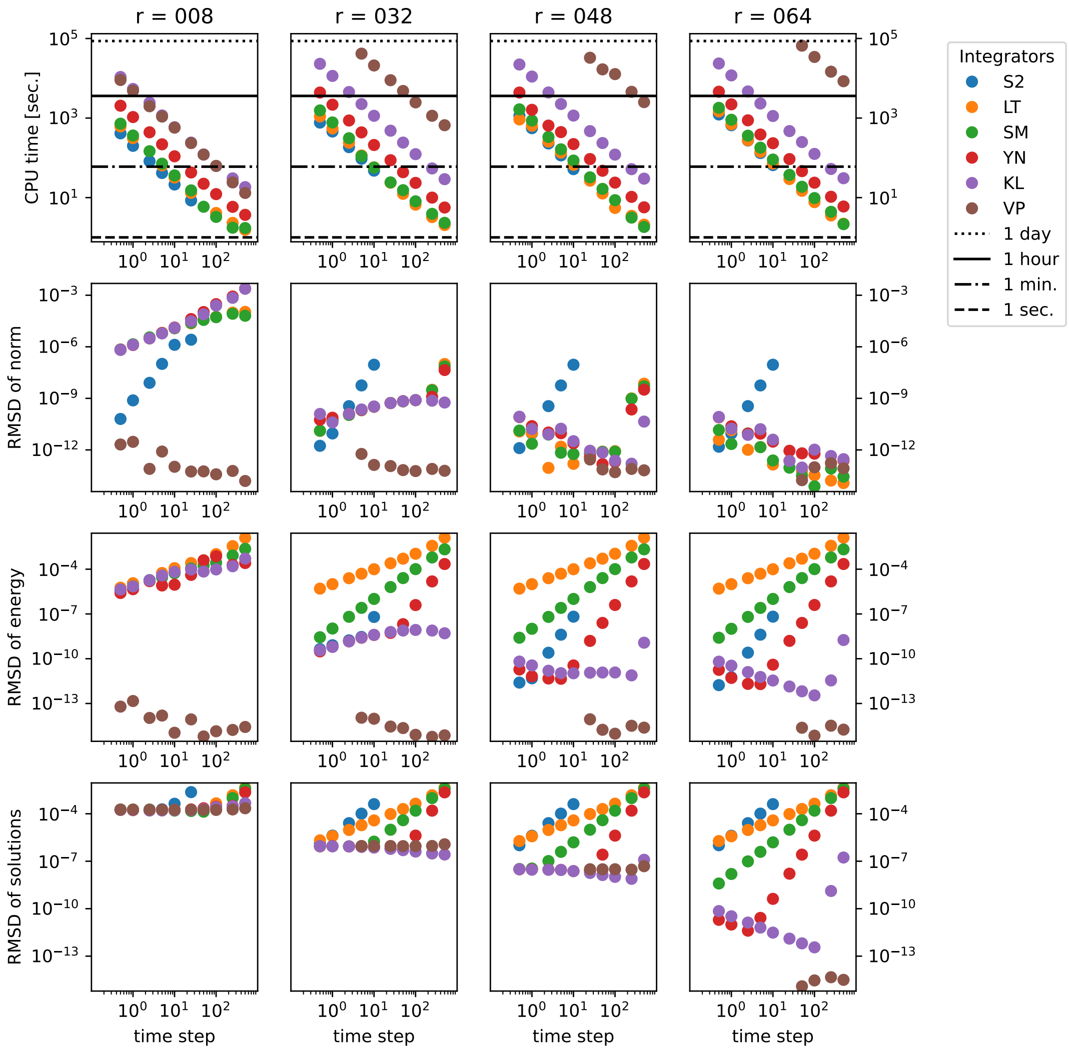


Figure 2. Quantum dynamics of purely phononic chains with $d = 8$ and $N = 4$ sites. For details, see caption of Fig. 1

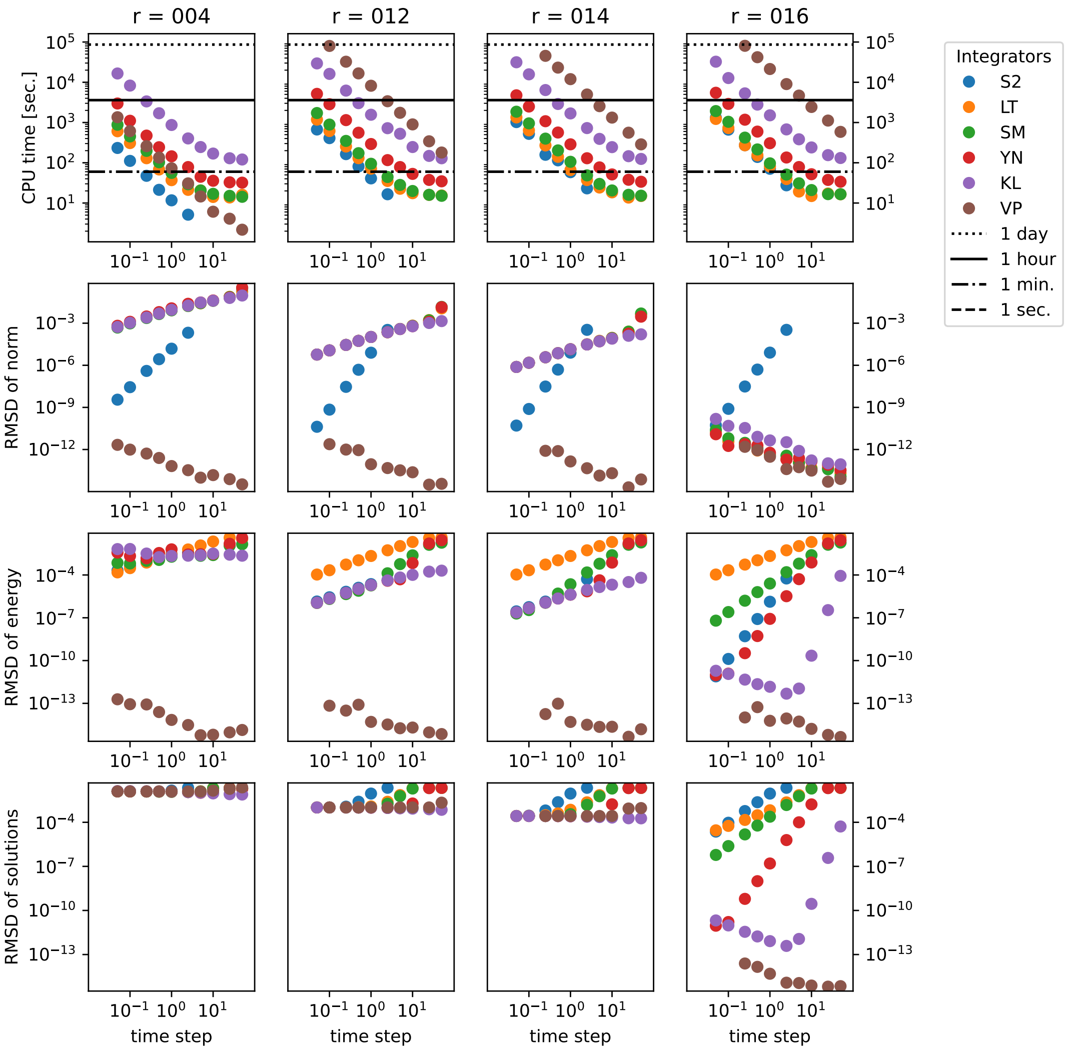


Figure 3. Quantum dynamics of coupled excitons and phonons for $d = 16$ and $N = 3$ sites. For details, see caption of Fig. 1

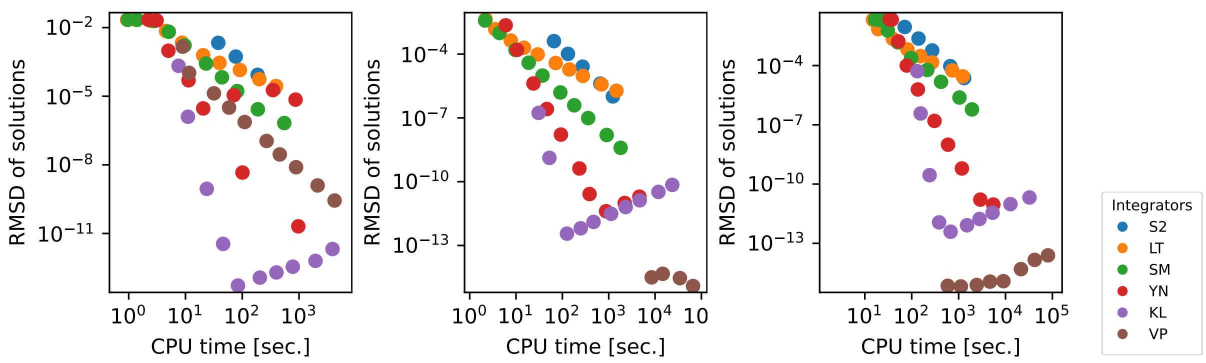


Figure 4. Accuracy of solutions versus computational effort. From left to right: excitons ($N = 12$, $r = 8$, $d = 2$), phonons ($N = 4$, $r = 64$, $d = 8$), and coupled systems ($N = 3$, $r = 16$, $d = 16$). For details, see caption of Fig. 1

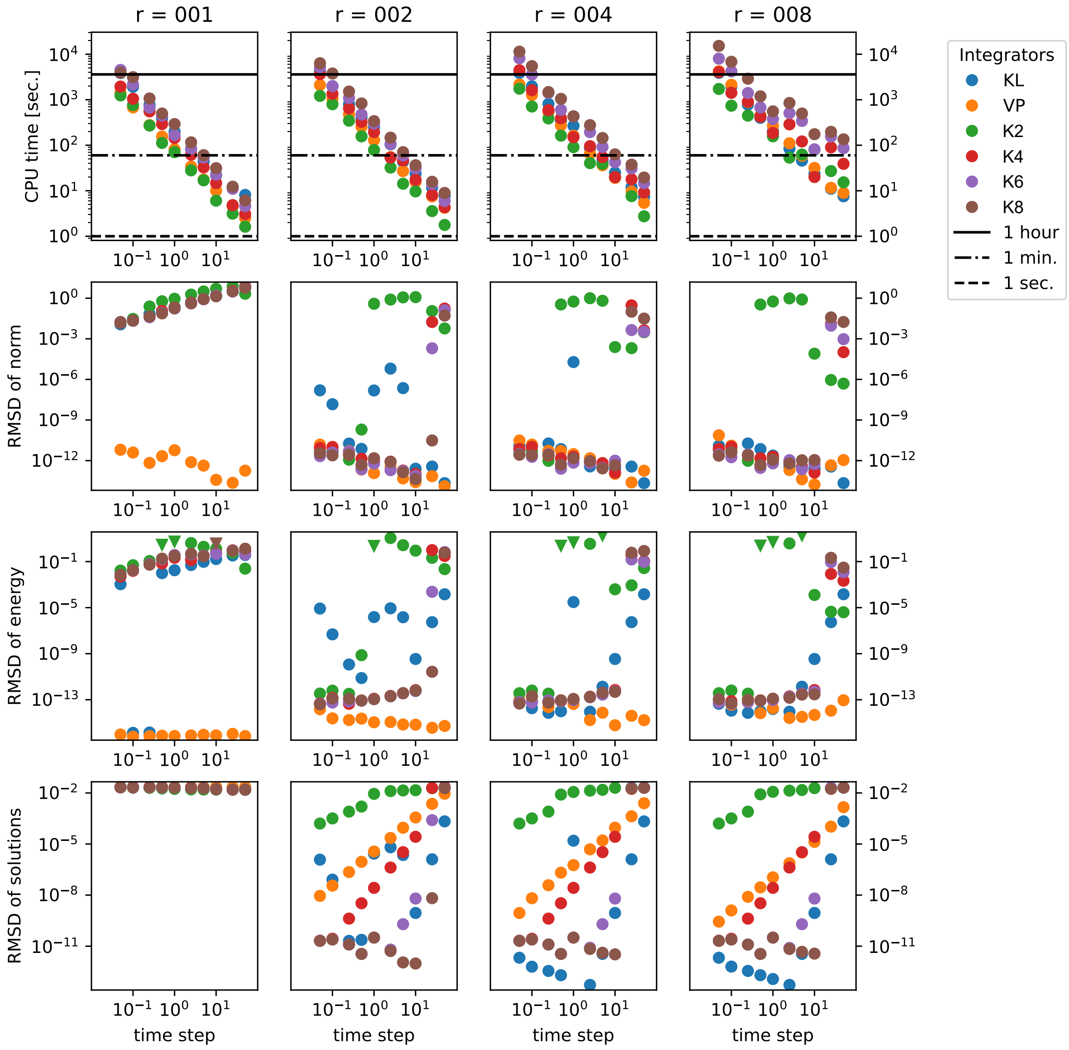


Figure 5. Quantum dynamics of purely excitonic chains with $d = 2$ and $N = 12$ sites. From left to right: Maximum number of ranks of state vectors increasing. From top to bottom: CPU-time versus size of temporal sub-steps, deviation of norm from unity, relative deviation of energy from initial value, deviation of state vectors from semi-analytical reference data. For 8th order Kahan-Li (KL), variational principle (VP), and various order global Krylov (K2, K4, K6, K8) integration methods

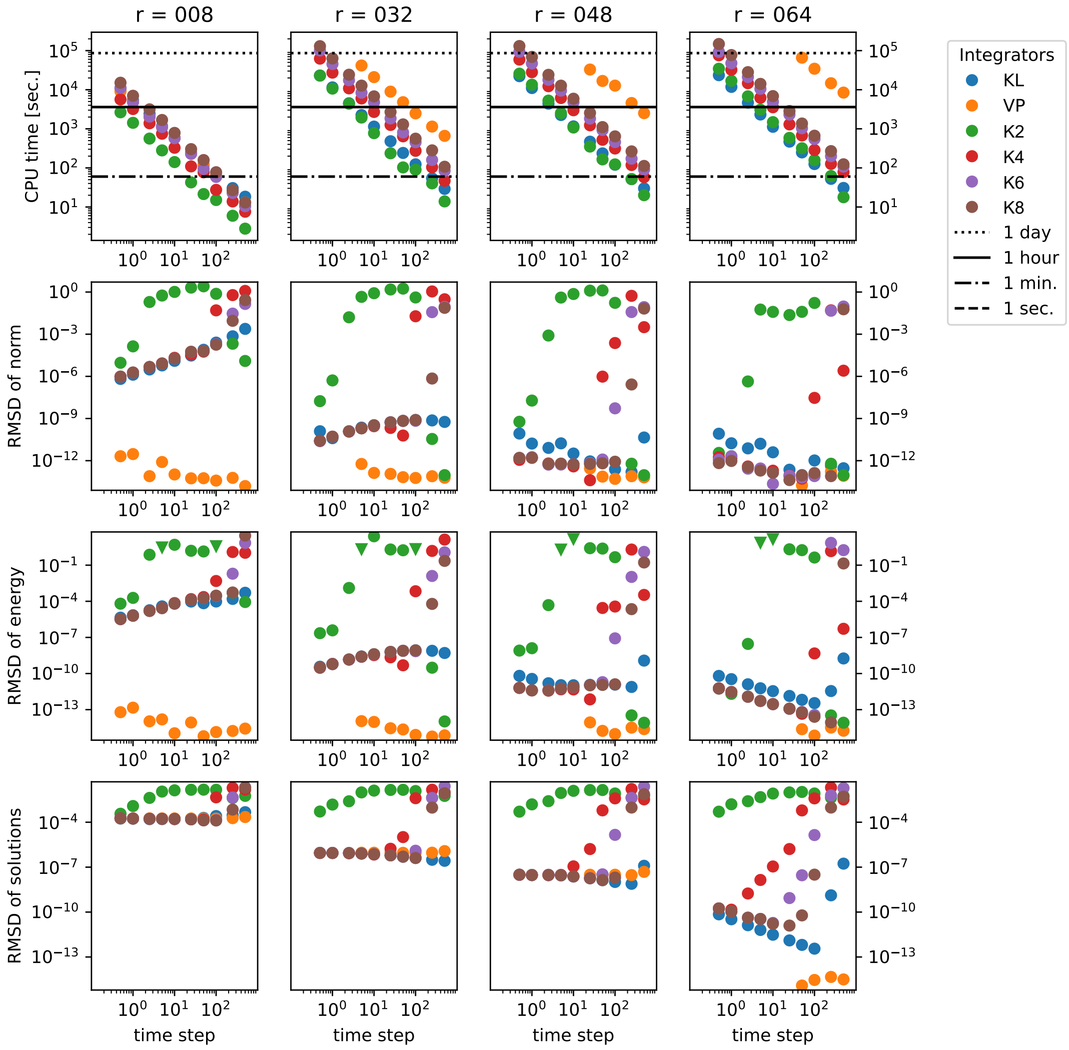


Figure 6. Quantum dynamics of purely phononic chains with $d = 8$ and $N = 4$ sites. For details, see caption of Fig. 5

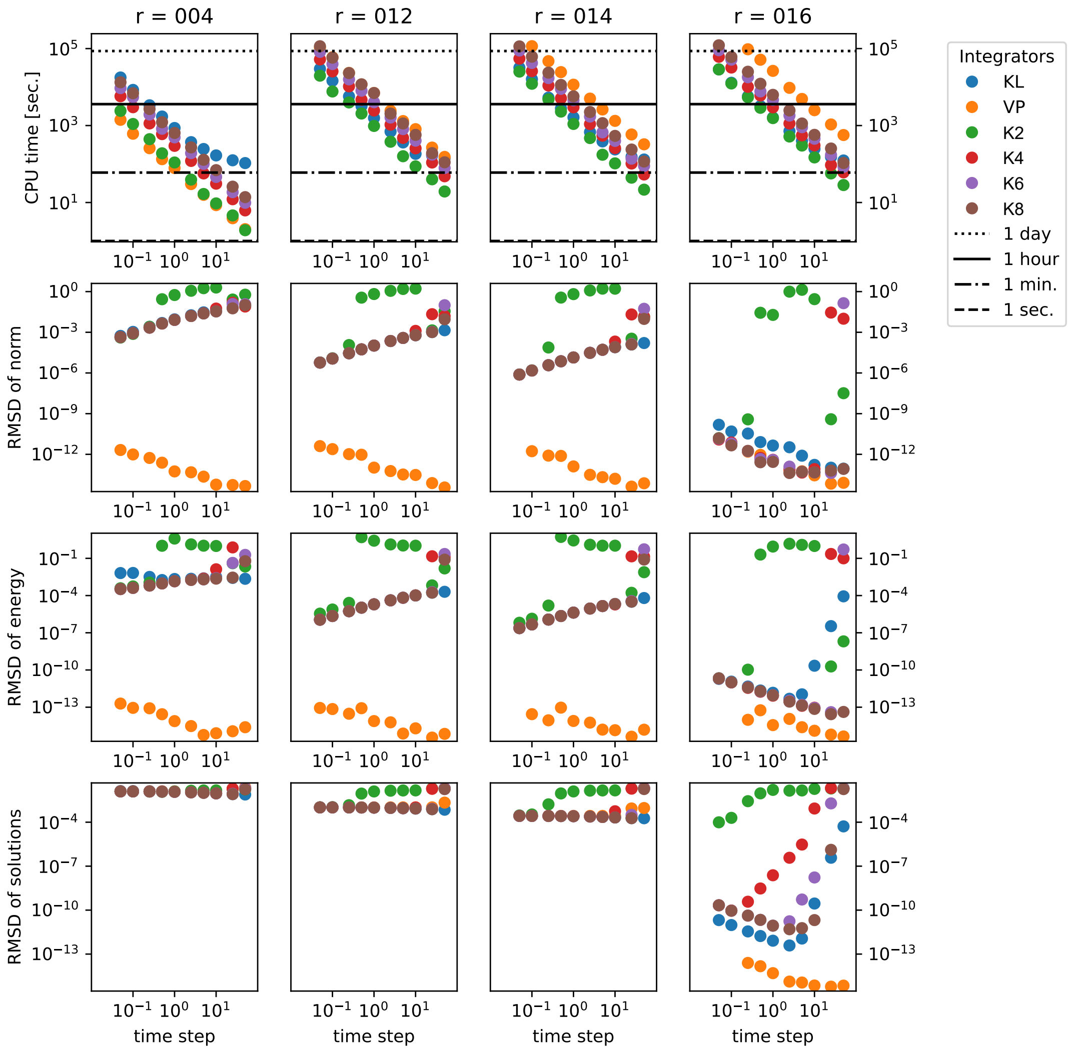


Figure 7. Quantum dynamics of coupled excitons and phonons for $d = 16$ and $N = 3$ sites. For details, see caption of Fig. 5
